# Supplementary material for: Imaging Dirac fermions flow through a circular Veselago lens
Source: arXiv:1811.02929 source file (2019-06-19)
Supplement: Supplementary file 1 [file Brun_supplemental.pdf]

# Imaging Dirac Fermions Flow Through a Circular Veselago Lens - Supplemental materials -

B. Brun[1], N. Moreau[1], S. Somanchi[2], V.-H. Nguyen[1], K. Watanabe[3], T. Taniguchi[3], J-C. Charlier[1], C. Stampfer[2] & B. Hackens[1]
[1]IMCN/NAPS, Université catholique de Louvain (UCLouvain), B-1348 Louvain-la-Neuve, Belgium
[2] JARA-FIT and 2nd Institute of Physics - RWTH Aachen, Germany
[3] National Institute for Materials Science, Namiki, Japan

June 19, 2019

## 1 Determination of the lever-arm

In order to convert the back gate voltage $V_{bg}$ into a charge carrier density $n_{2D}$, we need to evaluate the lever arm defined by $C = n/\Delta V$ where $\Delta V = V_{bg} - V_{CNP}$ with $V_{CNP} = -1$ V in our sample. This can be achieved by two different methods:

- From a simple capacitor model with $d_{h-BN} = 30$ nm and $d_{SiO_2} = 300$ nm, the lever-arm is $C = 6.1 - 6.7 \times 10^{14}\text{m}^{-2}\text{V}^{-1}$, depending on h-BN dielectric constant ($\epsilon_{\text{h-BN}} = 2 - 4$) [1].
- From Shubnikov-de Haas (SdH) oscillations, the Landau levels positions in the $(V_g, B)$ plane are given by the expression
$$B_\nu = \frac{\pi\hbar}{2e\nu} C\Delta V$$
where $\nu$ is the filling factor. By fitting the Landau levels positions in the conductance map in the $(V_g, B)$ plane (Fig. S1b), measured in the bulk of the sample (see Fig. S1a for the measurement configuration), we obtain $C = 7.4 \pm 0.2 \times 10^{14}$ $\text{m}^{-2}\text{V}^{-1}$.

## 2 Mobilities

Charge carriers mobilities are extracted from linear fits to the $G$ vs $n$ curve in the vicinity of the charge neutrality point (i.e. the Dirac cone). Note that we measure $G$ in the two-contacts configuration depicted in Fig. S1a, taking into account a total series resistance of 2 k$\Omega$ corresponding to the electrical filters on the measurement setup. This yields lower bounds for the mobilities : $\mu_e \sim 40\,000$ $\text{cm}^2\text{V}^{-1}\text{s}^{-1}$ for electrons and $\mu_h \sim 28\,000$ $\text{cm}^2\text{V}^{-1}\text{s}^{-1}$ for holes.

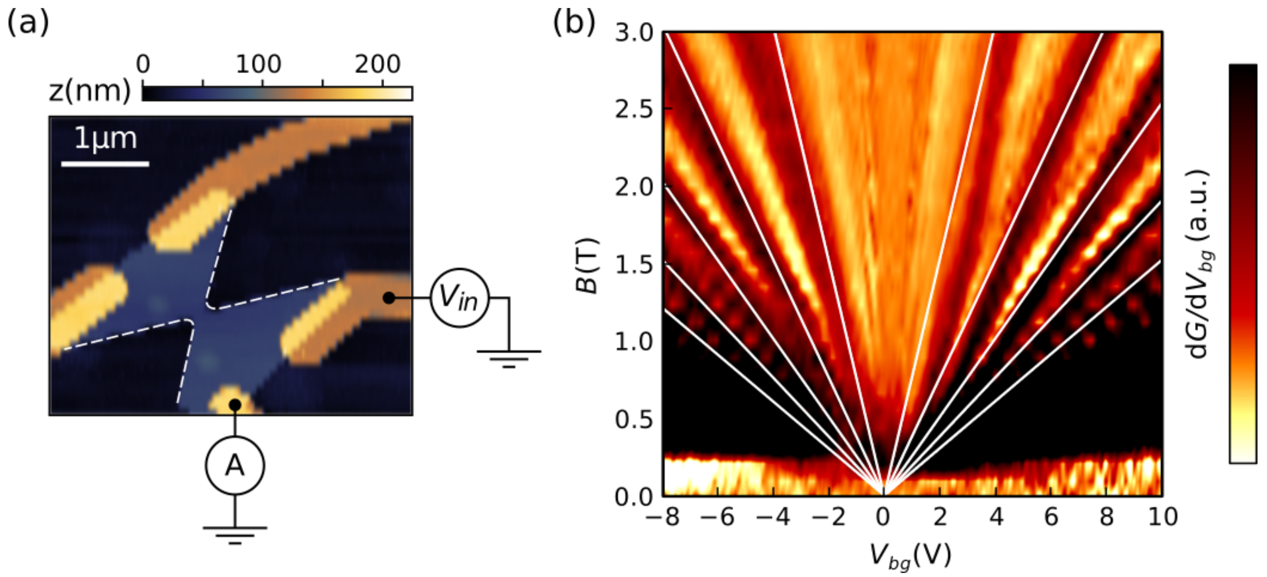


**Figure S1: Lever-arm parameter of the back-gate.** **(a)** AFM topography image of the graphene device. The two contacts used for the transconductance measurement shown in **(b)** are below the constriction, in yellow, and separated from each other by a distance of 800 nm. **(b)** Transconductance $\partial G/\partial V_{bg}$ as a function of $V_{bg}$ and $B$.

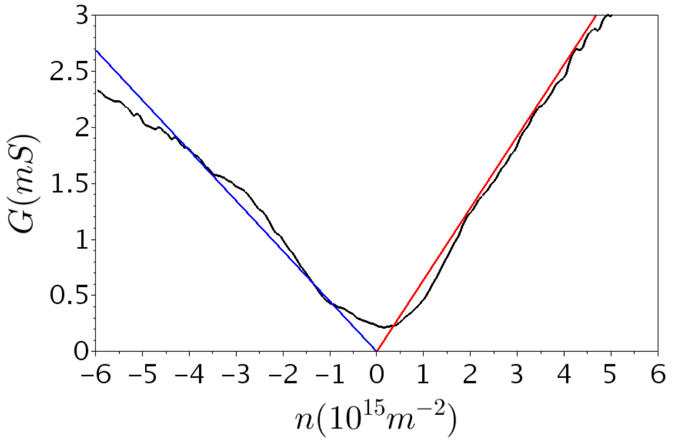


**Figure S2: Electron and holes mobilities from the Dirac cone slope.** Dirac cone measured in the same configuration as Fig. S1a. Two linear fits allow to calculate lower bounds for the electron and holes mobilities.

## 3 Temperature robustness

The main features of the SGM images discussed in the main text are visible at a temperature of ≈100 K. Fig. S3 shows SGM maps for a tip voltage of −8 V and a tip-to-graphene distance of

≈100 nm. The vertical as well as the horizontal length scales are only roughly estimated since we have no calibration for our piezoelectric scanner at 100 K. These images therefore just bring a qualitative insight on the temperature robustness of the observed features.

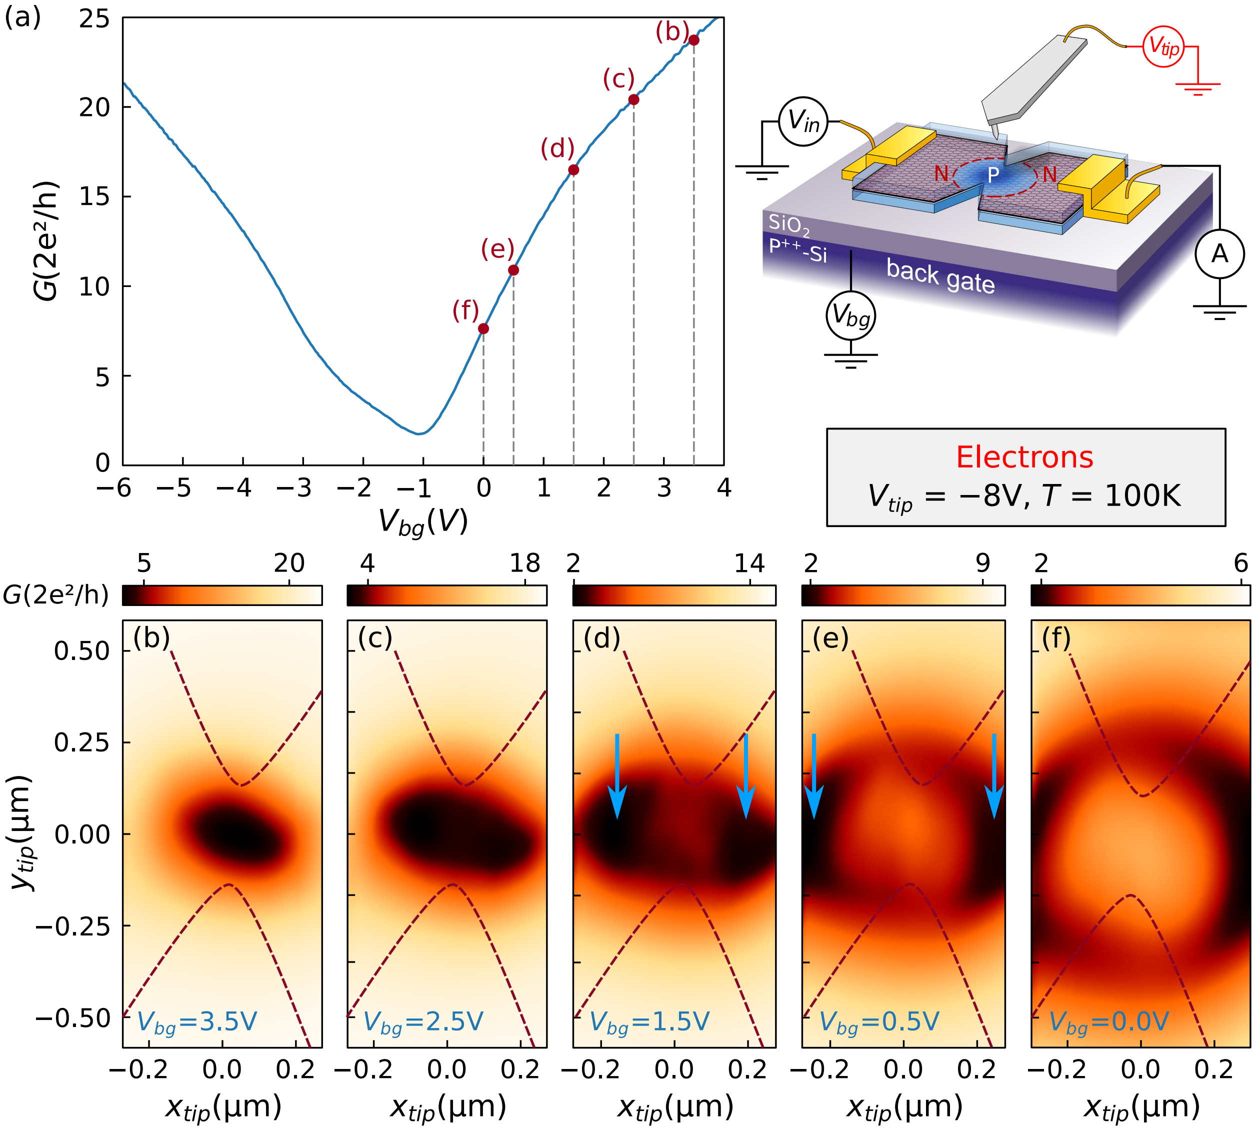


**Figure S3: Signatures of Veselago lensing at high temperature.** **(a)** $G$ vs $V_{bg}$ across the QPC, measured in four-contacts configuration, at a temperature around 100 K. **(b-f)** SGM maps for a tip voltage $-8$ V and tip-to-graphene distance of ≈100 nm, for the gate voltages indicated on (a).

# 4 Tip characterization

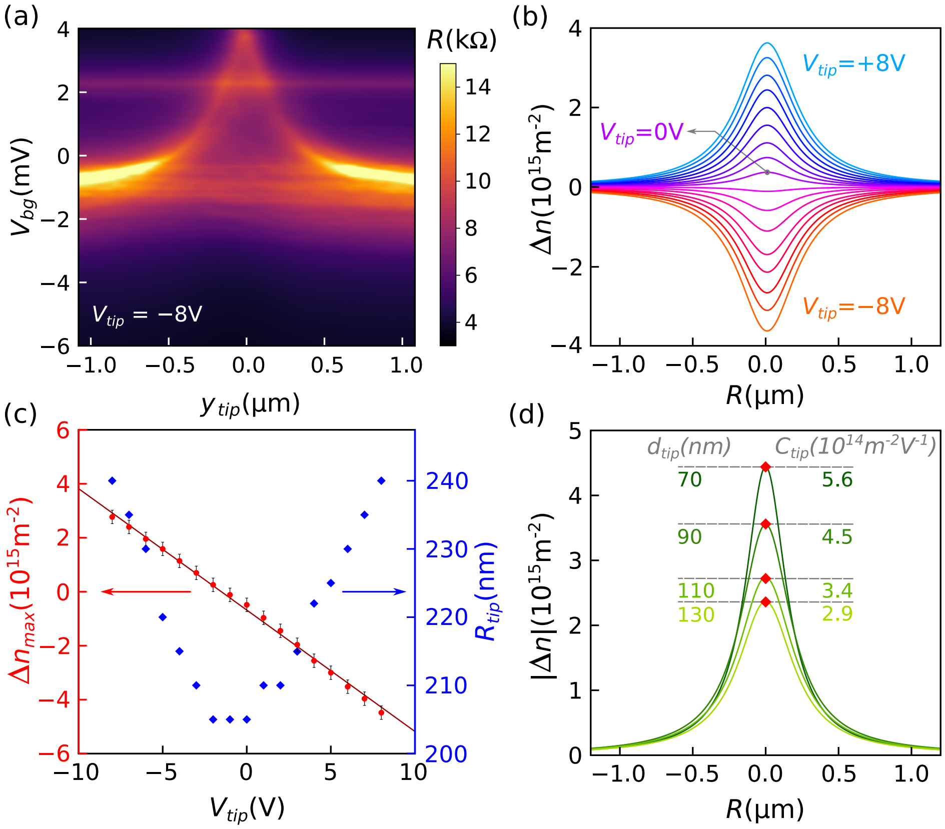


**Figure S4: Evaluation of the tip-induced potential. (a)** Resistance map as a function of tip position along a line passing by the centre of the constriction (position 0.0) perpendicularly to the transport axis, and $V_{bg}$. $d_{tip} = 90$ nm, $V_{tip} = -8$ V. **(b)** Fits of the tip-induced resistance maxima as a function of tip position extracted for different values of $V_{tip}$, from $-8$ V to $+8$ V, and $d_{tip} = 90$ nm, converted into local carrier density. **(c)** Evaluation of maximum charge density change around the center of the tip-affected region as a function of tip voltage (red points), and linear fit giving a tip lever-arm $C_{tip} = 4,5 \times 10^{14}$ m$^{-2}$V$^{-1}$(red line). $R_{tip}$, corresponding to half-width at half maximum of the Lorentzian fits in (b), as a function of $V_{tip}$ (blue dots). **(d)** Tip lever-arm parameter evolution with $d_{tip}$, for $V_{tip} = -8$ V

Fig. S4 presents the full characterization of the tip-induced potential for different tip voltages. As in the main text, we scan the tip along a line perpendicular to the QPC transport axis (red dashed line in Fig. 1a in the main text), and map the resistance $R$ as a function of back-gate voltage. The resulting figure exhibits a Lorentzian-shape maximum, as shown in Fig. S4a.

Horizontal lines can also be noticed in Fig. S4a, around $V_{bg} = +2.3$ V and $V_{bg} = -1$ V. The one at $V_{bg} = +2.3$ V corresponds to the contribution of the series ohmic contact responsible for the second Dirac cone also visible at $V_{bg} = +2.3$ V in Fig. 1c of the manuscript. It is therefore completely insensitive to the tip position along this specific line since this contact is far away from the scan line. The horizontal conductance minimum around $V_{bg} = -1$ V corresponds to the bulk

Dirac cone, i.e. away from the constriction.

Acquiring mappings similar to Fig. S4a, for different tip voltages at a fixed tip-to-graphene distance of 90 nm, yields the set of Lorentzian fits to the data displayed Fig. S4b.

In figure S4c we summarize these fits by plotting the maximum density change on top of the Lorentzian $\Delta n_{max}$ (red dots, right axis) and its half-width at half maximum $R_{tip}$ (blue dots, left axis). The maximum tip-induced density change as a function of tip voltage scales almost linearly with tip voltage, which allows us to characterize it by a simple lever-arm parameter $C_{tip} = 4.5 \times 10^{14}$ $\mathrm{m}^{-2}\mathrm{V}^{-1}$ for this tip-to-graphene distance.

# 5 Ruling out diffusive transport

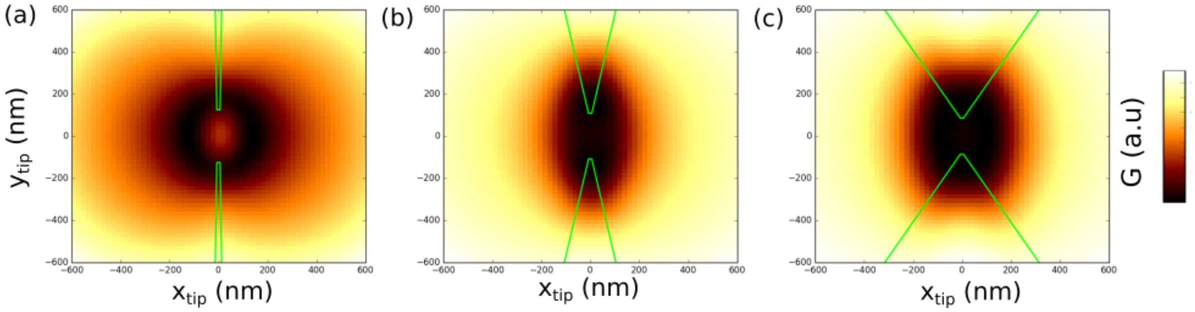


**Figure S5: Diffusive model:** (a) Total resistance calculated for a single opening dominating all the device resistance. The tip potential induces a change of carriers with a density change $\Delta n_{max} = -2 * n_{bulk}$. (b) Total resistance for a small opening angle constriction, with the same potential profile. (c) Total resistance for a constriction with a geometry corresponding to the experiment.

To check whereas diffusive transport could explain our observations, we study a simple one-dimensional model of the experiment, considering series resistance along the x-axis. Following early works on p-n junctions aiming at distinguishing between ballistic and diffusive transport [2], we assume a local conductivity $\sigma(x,y) = (\sigma_0^2 + [\mu e n(x,y)]^2)^{1/2}$, where $\sigma_0$ is the residual conductivity at the charge neutrality point, $n$ the local density, $\mu$ the mobility and e the electron charge. We then consider slices at abscissa $x$, that have a resistance $R(x)$ that depends on the density integrated over the y direction. The potential landscape is a Lorentzian similar to the one characterized in the manuscript, leading to a change in density $\Delta n_{max} = -2 * n_{bulk}$ at its maximum. The total conductance of the device is analyzed in this diffusive case, and plotted Fig.S5 as a function of tip position. FigS5a presents the case of a single aperture that would dominate the overall conductance of the device. In that case, a pattern that reminds the SGM maps observed experimentally is obtained, where the conductance when placing the tip at the center of the constriction is the same as when it is very far away. This is not surprising since the total resistance is given by the density at the constriction. However, considering the geometry of the experiment destroys this effect (Fig.S5c), because the openings of the constriction also contribute to the total resistance, and are affected by the tip too. The effect of the tip on the total transmission is more monotonic in that case, and the tip can only reduce the total transmission. This simple model shows that

diffusive transport alone cannot account for the observed behavior, and that ballistic trajectories and transmission and refraction laws at graphene p-n interfaces have to be taken into account.

# 6 Tight-binding simulations

In this section, we introduce briefly the tight-binding calculations [3] used to simulate the current density and the SGM maps presented in the main text (Fig. 4). Similar simulations have also been performed with the Kwant package [4] and led to the same conclusions.

The electronic properties of the considered graphene system are modeled by a first-nearest-neighbor tight-binding Hamiltonian [5]:

$$H = \sum_n V_n c_n^\dagger c_n + t \sum_{\langle n,m \rangle} c_n^\dagger c_m \tag{1}$$

where $t$ represents the hopping energy between first-nearest-neighbor $n^{th}$ and $m^{th}$ atoms and $V_n$ corresponds to the potential energy induced by gate voltages at the $n^{th}$ side. To compute the transport quantities, this tight-binding Hamiltonian is solved using the Green's function technique [3]. In particular, the retarded Green's function is determined as:

$$\mathcal{G}(E) = \left[E + i0^+ - H - \Sigma_L - \Sigma_R\right]^{-1}, \tag{2}$$

where $\Sigma_{L,R}$ are the self-energies describing the left and right device-to-lead couplings, respectively. This Green's function equation is solved using the recursive method [6]. The transport quantities such as conductance and bond currents injected from the left lead are then computed using the following formulas:

$$G(E_F) = \frac{2e^2}{h} Tr\left[\Gamma_L \mathcal{G} \Gamma_R \mathcal{G}^\dagger\right], \tag{3}$$

$$J_{nm}^L(E_F) = -\frac{2e}{h} H_{nm} Im\left(\mathcal{G}\Gamma_L\mathcal{G}^\dagger\right)_{nm} \tag{4}$$

with $\Gamma_{L,R} = i\left(\Sigma_{L,R} - \Sigma_{L,R}^\dagger\right)$.

In order to simulate graphene devices of similar sizes (i.e., at the $\mu$m scale) as in the experiments, there is however a numerical challenge. In particular, the simulation of such large graphene system (typically, more than 8000 lattice sites in transverse direction for W = 1 $\mu$m) includes several million carbon orbitals. Hence, to avoid such numerical challenge, we employed the scaling technique as presented in [7], that has been demonstrated to work very well for graphene device simulations. In particular, we increase the bond length $a_{CC}$ between the carbon atoms by a factor of $s_f$ = 24 (i.e., $a_{CC} = s_f a_0$ where $a_0 = 0.142$ nm is the well known $C - C$ bond length in graphene) and simultaneously decreases the nearest neighbor hopping energy with the same factor (i.e., $t = t_0/s_f$ where $t_0 = 2.7$ eV is the typical tight-binding hopping energy [5]).

# 7 Anti-focusing with a constriction

In the main text, we study the appearance of low conductance spots (low $G$ spots) in the experimental SGM maps. In order to understand the origin of these spots, we compare simulated SGM

maps (Fig. S6a) with current density maps simulated in a graphene sheet without constriction (Fig. S6b). In this section, we detail how to interpret the SGM map in relation to the current density map. In particular, we will explain why the low $G$ spots (blue arrows in Fig. S6a) do not have exactly the same shape as the low current density spots (low $\vec{J}$ spots, red arrows in Fig. S6b). Section 8 presents some perspectives towards getting a direct correspondence between the SGM maps and the current density around a p-n junction.

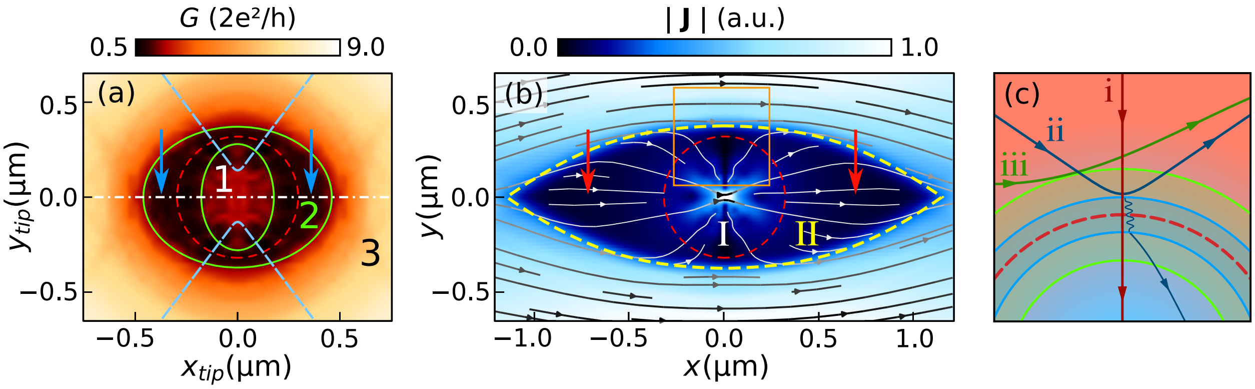


**Figure S6: Comparison between simulated current density and SGM maps. (a-b)** Same SGM maps as Fig. 4d and 4c in the main text. Different zones have been delimited on top of the maps for the discussion exposed in the text. Blue arrows indicate the position of the low $G$ spots and red arrows indicate the position of the low $\vec{J}$ spots. **(c)** Qualitative sketch illustrating the electron trajectories (i, ii and iii) impinging the circular smooth p-n junction in an area corresponding to the orange square in (b). A *forbidden zone* is associated to each trajectory (blue boundaries for trajectory ii and green for iii).

To properly understand the SGM maps, we performed simulations using our home-made code presented in section 6. Figure S7 shows simulations of the current density in a large graphene ribbon containing a constriction whose width is progressively lowered. The tip potential used in each figure is the same as in Fig. 4c-d of the main text. All the current density maps are normalised with the same factor $J_{max}$ so they can be compared together.

Figure S7a shows a map of the current density in a ribbon without constriction that exhibits the two characteristic low $\vec{J}$ spots. These spots are caused by the smooth p-n junction that bends the electrons trajectories. When the constriction width is lowered (Fig. S7b-e), the edges of the constriction also bend electrons trajectories towards the centre of the constriction. The conductance is therefore given by the combined influence of the tip potential and the constriction. The important feature observed in Fig. S7b-e is the reduction of the low $\vec{J}$ spot size as the constriction width is lowered. This explains why the low $G$ spots do not directly map the low $\vec{J}$ spots.

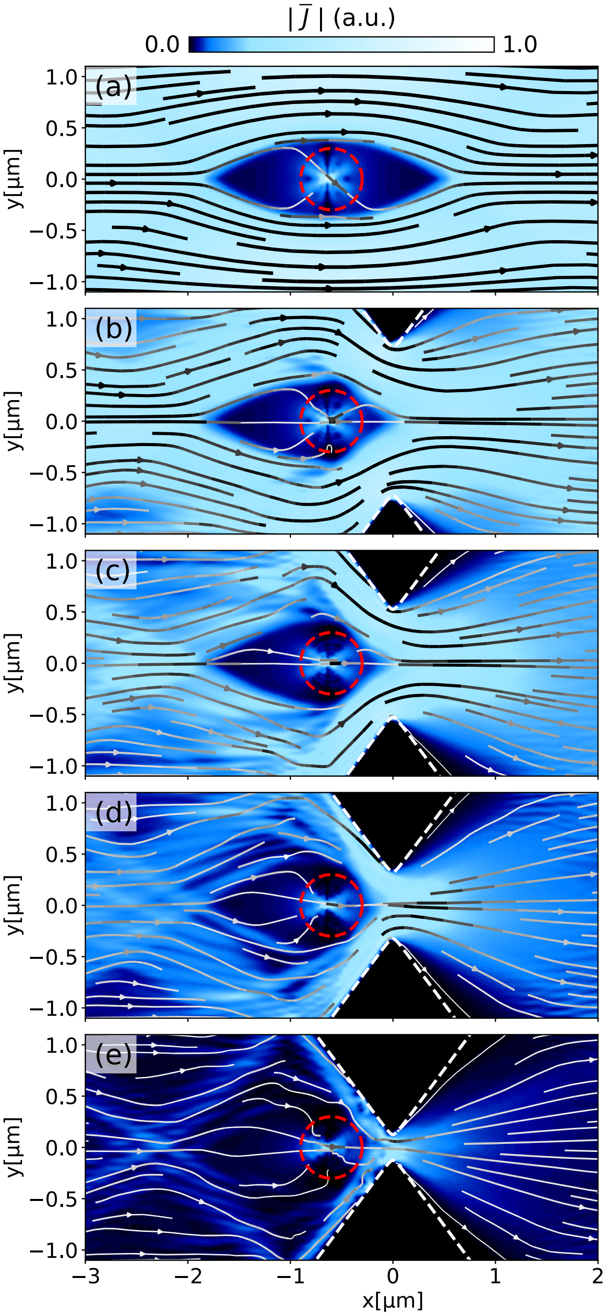


**Figure S7: Simulation of current density when varying the constriction width.** A Lorentzian potential ($V_m = 2E_F$) creates a circular p-n junction (red dashed line, $R_{tip} = 300$ nm). **(a)** Current density computed without constriction. Two spots of low current density appear, similarly to figure S6a. **(b-e)** Current density computed for constriction widths of respectively : **(b)** 1450 nm, **(c)** 1050 nm, **(d)** 650 nm and **(e)** 250 nm. The distance between the tip and the constriction is 600 nm.

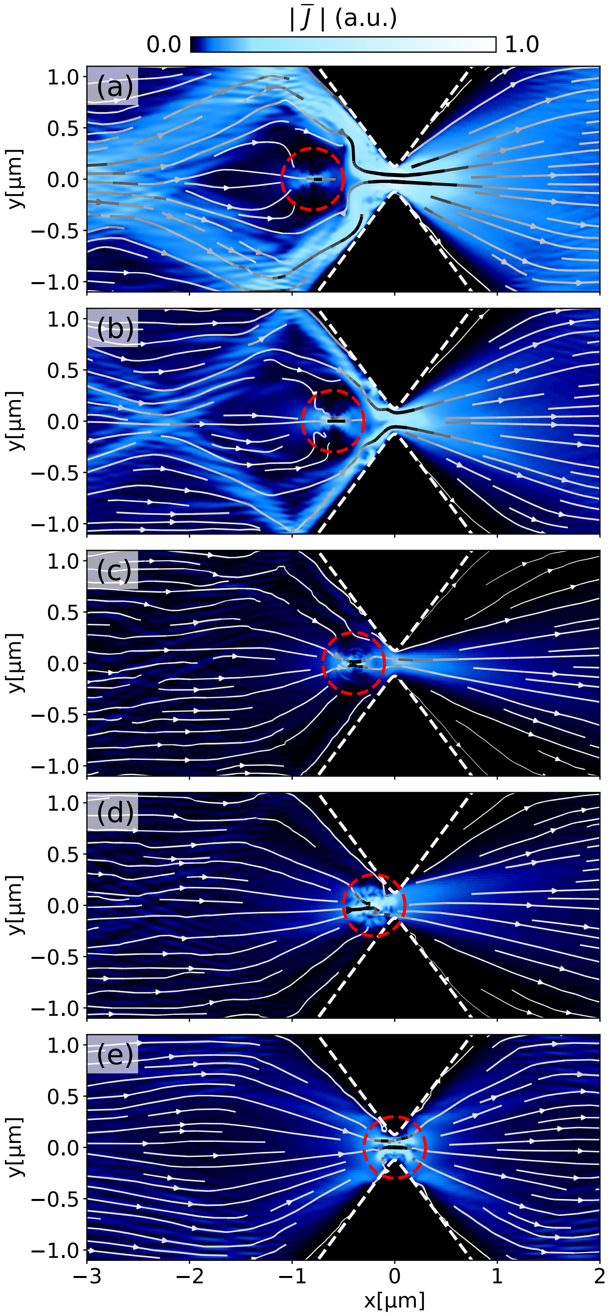


**Figure S8: Simulation of current density when varying the tip position.** A Lorentzian potential ($V_m = 2E_F$) creates a circular p-n junction (red dashed line, $R_{tip} = 300$ nm). The tip position is moved along $x$ and is located at a distance from the constriction of **(a)** 800 nm **(b)** 600 nm, **(c)** 400 nm, **(d)** 200 nm and **(e)** 0 nm. The width of the constriction is 250 nm.

With the bending effect of the edges in mind, we can discuss the origin of the low $G$ spots. Figure S8 illustrates the influence of the tip potential on the conductance for a constriction of 250 nm. The tip potential is the same as the one used in Fig. S7 and Fig. 4c-d . We can distinguish four situations:

1. When the tip is far from the centre of the constriction (Fig. S8a), electrons flow along the edges. The low $\vec{J}$ spot at the constriction side disappears and the conductance remains high.

2. When the tip starts to get closer to the constriction (Fig. S8b), the trajectories along the edges encounter the p-n junction with a parallel incidence. Due to the junction smoothness, a *forbidden zone*[1] (illustrated in Fig. S6c) appears, whose width depends on the incident angle of the electron trajectories [8]. For parallel incidence (trajectory iii in Fig. S6c), the forbidden zone (delimited by green boundaries) is wide. By approaching the tip from the edge, the forbidden zone starts to block edge trajectories, reducing the conductance.

3. When further approaching the tip (Fig. S8c and d), the majority of trajectories will be blocked due to the effect of the forbidden zone around the p-n junction. Only the trajectories favoured by Klein tunnelling will go through the constriction. In this configuration, the transmission mainly depends on the constriction width and the p-n junction shape, as it will be illustrated in section 8.

4. Finally, when the tip is located at the centre of the constriction (Fig. S8e), the conductance is dominated by Klein tunnelling so that the transmission increases again. This is illustrated by trajectory i in Fig. S6c.

Since we have a good insight about the mechanisms at play when the tip approaches the constriction, we can summarise by establishing the correspondence between the SGM map of Fig. S6a and the current density map of Fig. S6b. To do so, the SGM map and the current density map have been divided into different zones in Fig. S6.

- **Zone 1** corresponds to an increase of the conductance. It is a direct consequence of the high current density in the lens core indicated by **zone I**. This region is therefore an image of Klein tunnelling in real space.

- **Zone 2** and **zone II** are a consequence of the smoothness of the junction. Zone 2 has its origin in the forbidden zone that blocks electron trajectories in the vicinity of the constriction, as discussed above in point 3. Zone II is also related to the presence of the forbidden zone. Indeed, only perpendicular trajectories cross the p-n junction. The smoothness of the potential also bends the trajectories, leading to the stretched shape of zone II along transport axis.

- **Zone 3** in Fig. S6a is given by potential positions that are far from the constriction center so that the perturbation has only a weak effect on the electron transmission.

Even if they are both due to the smoothness of the potential, zone 2 does not directly map zone II. Indeed, as highlighted in Fig. S7 and the related discussion, the bending of the electron trajectories, due to the constriction, suppresses the low $\vec{J}$ spots. In section 8, we will see how the constriction geometry can be modified to map zone II in a SGM map.

[1] By *forbidden zone*, we mean a zone that electrons can only cross by tunnelling (with a decaying exponential transmission), as illustrated by trajectory ii in Fig. S6c [8]

## 8 Constriction as a current density detector

In section 7, the origin of the low $G$ spots in the SGM maps has been discussed. They are due to the effect of the smooth p-n interface that blocks the transmission of electrons when it is in the vicinity of the constriction. Due to the bending of the electron trajectories by the constriction edges, the low $G$ spots do not have exactly the same shape as the low $\vec{J}$ spots. In this section, we will detail how the design of the constriction can be modified in order to obtain a direct correspondence between the SGM map and the current density map without constriction. To do so, a constriction defined by vertical (i.e; perpendicular to the transport axis) boundaries is studied, as depicted in Fig. S9a. The constriction opening width, along $y$, is 250 nm and its length, along $x$, is 60 nm.

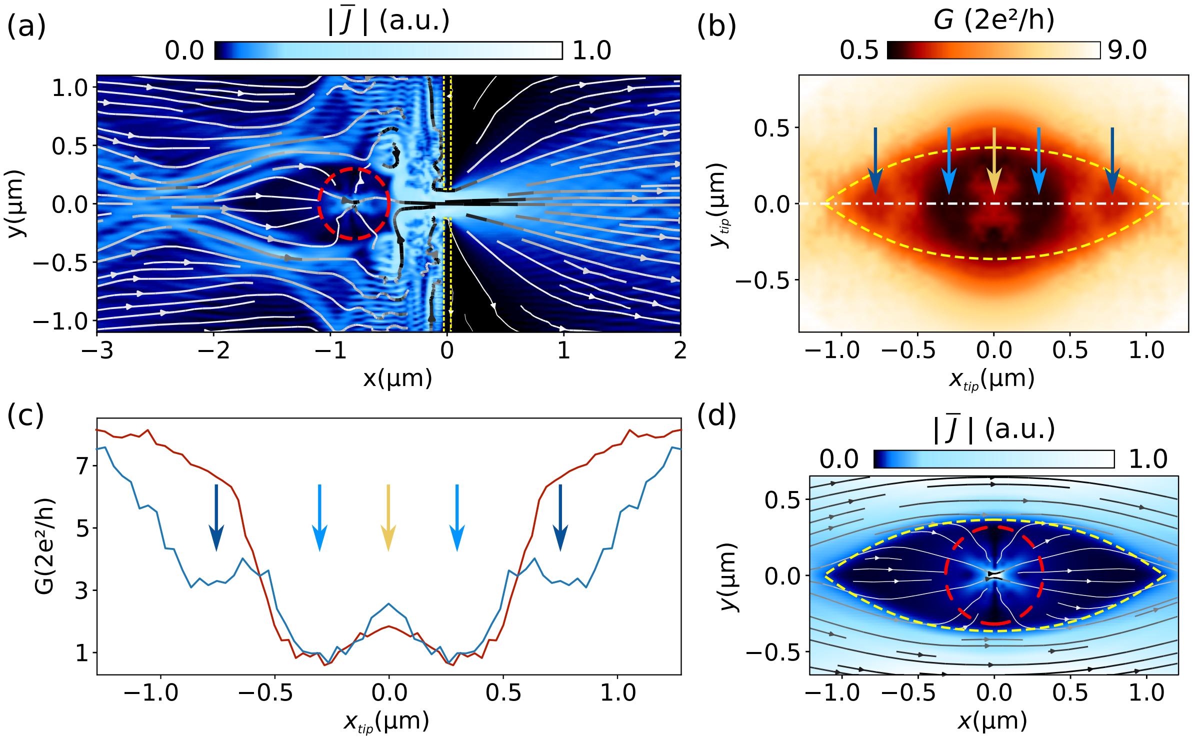


**Figure S9: Effect of the constriction shape on the SGM maps. (a)** Current density map in a constriction defined by vertical boundaries (yellow dashed line) in presence of a Lorentzian potential ($V_m = 2E_F$) that creates a circular p-n junction (red dashed line, $R_{tip} = 300$ nm). **(b)** SGM map in the same constriction and for the same Lorentzian potential as (a). The yellow dashed line shows the limits of the low current density zone shown in (d). **(c)** Blue curve: conductance at $y_{tip} = 0$, obtained along the white dash-dotted line of (b). Red curve: conductance curve at $y_{tip} = 0$, obtained along the white dash-dotted line of Fig. S6a. The arrows show three characteristic zones of the SGM map. **(d)** Same figure as Fig. S6 and Fig. 4c in the main text. The yellow dashed line delineates the low current density zone.

The SGM map obtained in the new constriction geometry is shown in Fig. S9b. It can be compared to the map ′of Fig. S6a obtained for the previous constriction geometry. Fig. S9c shows

line cuts at $y_{tip} = 0$ in the two SGM maps. The obtained conductance curves highlight the key differences between the two geometries. Three zones can be distinguished, indicated by arrows in Fig. S9b and c:

- The **gold arrow** indicates the zone of increased conductance caused by Klein tunnelling. This is the zone 1 discussed in section 7.
- **Light blue arrows** indicate the low $G$ spots described by zone 2 in section 7. The position and the shape of these spots are rather similar for both constriction geometries, as highlighted in Fig. S9c. The shape of the low $G$ spots therefore mainly depend on the constriction width and the effect of the p-n interface. The slope of the constriction boundaries will also slightly modify the shape. Indeed, the p-n interface will not reach the constriction edges at the same distance from the constriction center (see Fig. S8 and the related discussion - point 2). The conductance will therefore not fall at the same position, as illustrated in Fig. S9c.
- **Dark blue arrow** indicate plateaus of reduced conductance only visible for the vertical boundaries (blue curve in Fig. S9c). By comparing Fig. S9b and d, it appears that these zones of reduced conductance are directly related to the low $\vec{J}$. To emphasise this correspondence, the delimitation of the low $\vec{J}$ zone (yellow doted line in Fig. S9d) is reported on Fig. S9b.

The appearance of this last zone, for the vertical boundaries, can be explained by a less efficient bending of electron trajectories toward the center of the constriction, compared to the oblique edge (see section 7). Indeed, the vertical edges will mostly back-scatter electrons instead of bending their trajectories as illustrated by Fig. S9a (in comparison to Fig. S8). The low $\vec{J}$ spots (zone III in Fig. S6) have therefore a real influence when the potential is in front of the constriction. This explains the good correspondence between Fig. S9b and d.

To conclude, the shape of the constriction plays an important role on the SGM data. By designing properly this constriction, it can be optimised to yield features that directly correspond to the current density around a tip-induced potential. This opens the way to new devices for SGM characterisation.

## 9 Turning off Klein tunneling and Veselago lensing

To get more clue about the role of graphene peculiar properties in our experiment, we modeled gapped graphene, by considering theoretically graphene aligned with a Boron-Nitride substrate. We induce a small gap compared to the energies in the p and n region, such that the local density of states is still high in both the p and n regions, as shown Fig. S10 f. This gap however prevents Klein tunneling and Veselago lensing effects. The effect on the current density is the disappearance of the high $|\vec{J}|$ region at the lens core (Fig. S10 g). Concomitantly, the spot of high conductance when placing the lens at the center of the constriction disappears in the case of gapped graphene, as visible by comparing the SGM images Fig.S10g (normal graphene) and S10h (gapped graphene).

This demonstrates that the SGM images indeed reflect the current density through the p-n junction, and not only the local density of states, or local conductivity. Though based on a different physical system, these calculations show that the perfect transmission between the p and n regions is crucial to obtain the effect observed experimentally. This high transmission is achieved thanks

to Klein tunneling, which is at play in our experiment, and appears as a necessary ingredient to understand the observed behavior.

It is however difficult to quantify the contributions from Veselago lensing and from Klein tunneling, as they're indeed different manifestations of the same phenomenon. The Veselago lensing effect denotes Klein tunneling at a finite incidence angle. In our experiment, the pn interface is circular, which offers a large variety of incident angles compared to planar interfaces used in previous experiments[9, 10]. By collecting different incident angles and refocusing them at the same point, our geometry therefore favors the effect of Veselago lensing compared to "normal" Klein tunneling.

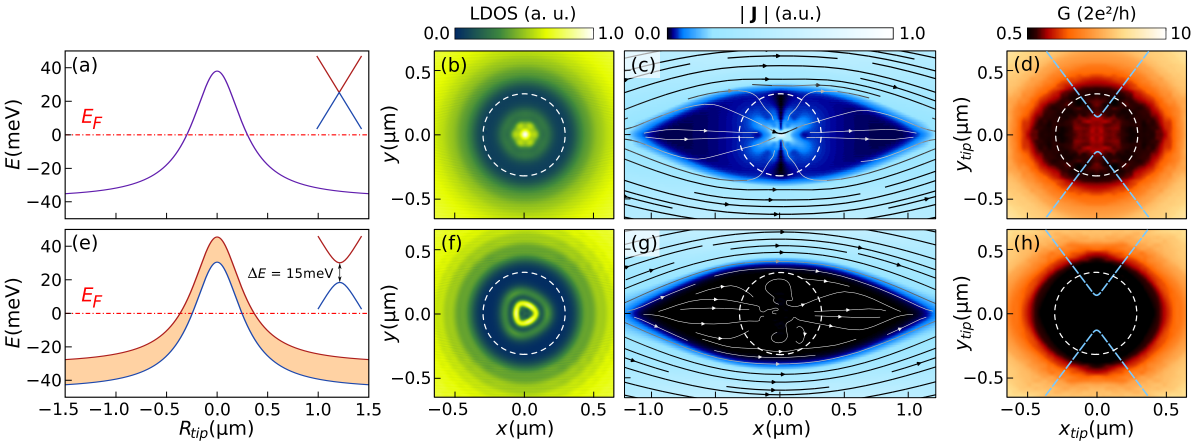


**Figure S10: Turning off Klein tunneling with gapped graphene:** (a) Potential profile used to calculate transport through graphene pn junction. (b) Local density of state (LDOS) for normal graphene in the circular pn junction. (c) Local current density for normal graphene. (d) SGM map expected when scanning the perturbation around a constriction. (e) Potential profile used in the case of gapped graphene. (f) LDOS for a gapped graphene p-n junction. (f) $|\vec{J}|$ in for gapped graphene. (h) SGM image computed for gapped graphene.

## 10 Effect of the junction smoothness

In this section, we present the current density and SGM maps for different decay exponent $d$ of the tip-induced potential $V(\vec{r}) = \frac{V_m}{1+\left(\frac{\|\vec{r}-\vec{r}_{tip}\|}{R_{tip}}\right)^d}$.

In Fig.S11, the effect of the junction smoothness on both the current density and the SGM maps is clarified. Fig.S11(c-f) correspond to the Lorentzian (d=2) and abrupt (d=∞) potential profiles already presented in Fig.4 of the manuscript. Fig.S11g and h present the intermediate case of a potential that decays faster than a Lorentzian but still evolving smoothly (d=5). The distance of the anti-focusing points evolve in both the current density and he SGM maps. Finally, Fig.S11 a and b present $\vec{J}$ and the SGM map in the n-n'-n configuration, where the density below the tip reaches the charge neutrality in a single point.

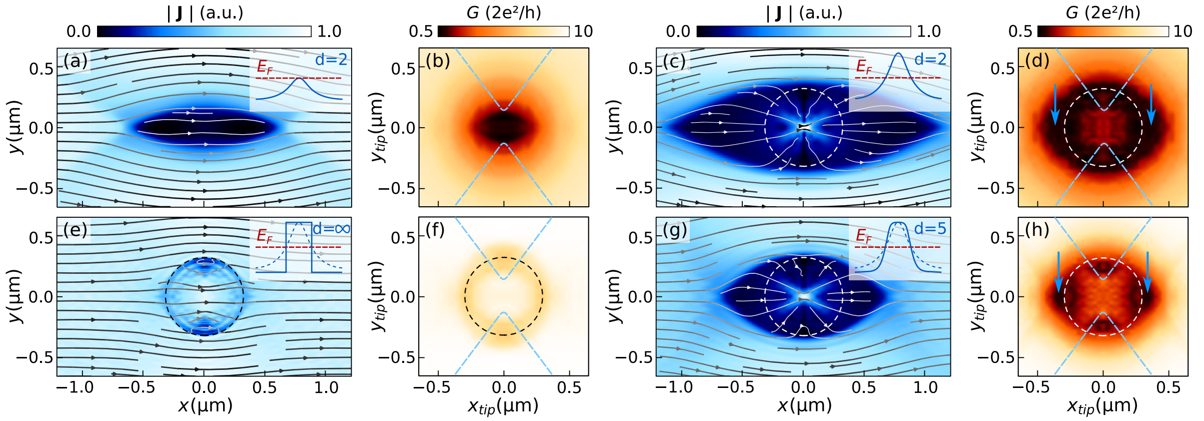


**Figure S11: Influence of the junction smoothness:** Simulations of current density $\vec{J}$ in a graphene sheet around the fixed tip potential of Eq. (**??**) characterized by the parameters $V_m$, $E$ and $d$ (left image in each couple), and simulated SGM maps obtained by displacing the same potential around a 250 nm-wide constriction (right image in the couple). (a-b) Lorentzian profile ($d = 2$) with $V_m = E$. (c-d) n-p-n configuration with $d = 2$ and $V_m = 2E$. (e-f) Abrupt circular p-n junction with $d = \infty$ and $V_m = 2E$. (g-h) Fast decaying potential profile ($d = 5$) with $V_m = 2E$. The chosen energy $E$ corresponds in all cases to $n = 1.5 \times 10^{15}\text{m}^{-2}$, and $\Delta n_{max} = -3 \times 10^{15}\text{m}^{-2}$ in (c) to (h). Dashed circle indicates the *locus* corresponding to zero charge density. Insets: schematics of potential profile vs position, Lorentzian profile is indicated as dashed blue line for comparison, when $d \neq 2$.

## 11 Fabry-Pérot interference

In Fig.S12(a), we plot the conductance as a function of $V_{tip}$ of $V_{bg}$, recorded at 4K by placing the tip at the center of the constriction, 70 nm above the sample surface. Clear oscillations are visible in the n-p-n and p-n-p configurations, due to Fabry-Pérot interference. The series ohmic contact resistance peak is visible at $V_{bg} \simeq 2.5$ V and is insensitive to tip voltage since this contact is situated far away from the constriction. It can hence clearly be distinguished from the Fabry-Pérot interferences. These interferences are at the moment under deeper investigation and will be detailed in another paper.

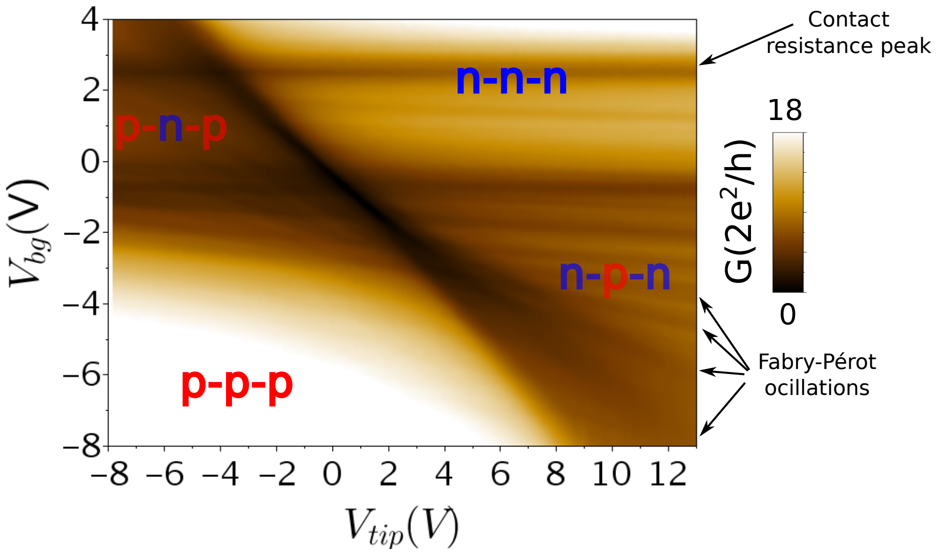


**Figure S12: Fabry-Pérot interference:** Conductance G as a function of tip voltage $V_{tip}$ and back-gate voltage $V_{bg}$, when placing the tip at the center of the constriction, at a distance $d_{tip}$ = 70 nm from the sample surface.

# References


[1] K. K. Kim *et al.*, *Synthesis and characterization of hexagonal boron nitride film as a dielectric layer for graphene devices*, ACS Nano **6**, 8583 (2012)

[2] B. Huard *et al.*, *Transport Measurements Across a Tunable Potential Barrier in Graphene*, Phys. Rev. Lett. **98**, 236803 (2007)

[3] V. H. Nguyen *et al.*, *Bandgap nanoengineering of graphene tunnel diodes and tunnel transistors to control the negative differential resistance*, J. Comput. Electron. **12**, 85 (2013)

[4] C. W. Groth *et al.*, *Kwant: a software package for quantum transport*, New J. Phys **16**, 063065 (2014)

[5] A. H. Castro Neto *et al.*, *The electronic properties of graphene*, Rev. Mod. Phys. **81**, 109 (2009)

[6] C. H. Lewenkopf *et al.*, *The recursive green's function method for graphene*, J. Comput. Electron. **12**, 203 (2013)

[7] M.-H. Liu *et al.*, *Scalable tight-binding model for graphene*, Phys. Rev. Lett. **114**, 036601 (2015)

[8] V. V. Cheianov and V. I. Fal'ko, *Selective transmission of Dirac electrons and ballistic magnetoresistance of n-p junctions in graphene*, Phys. Rev. B **74**, 041403(R) (2006)

[9] G.-H. Lee, G.-H. Park, and H.-J. Lee, *Observation of negative refraction of Dirac fermions in graphene*, Nature Physics **11**, 925 (2015).

[10] S. Chen *et al.*, *Electron optics with p-n junctions in ballistic graphene*, Science **353**, 1522 (2016).
